# Supplementary material for: Weak equilibria for time-inconsistent control: with applications to investment-withdrawal decisions
Source: arXiv:2105.06607 source file (2023-06-17)

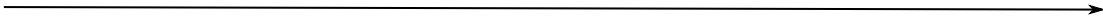

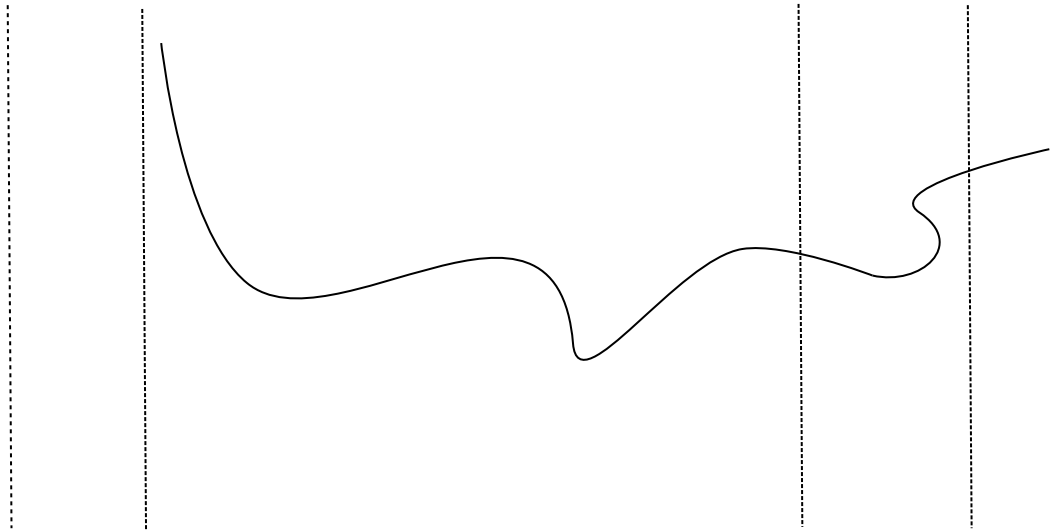

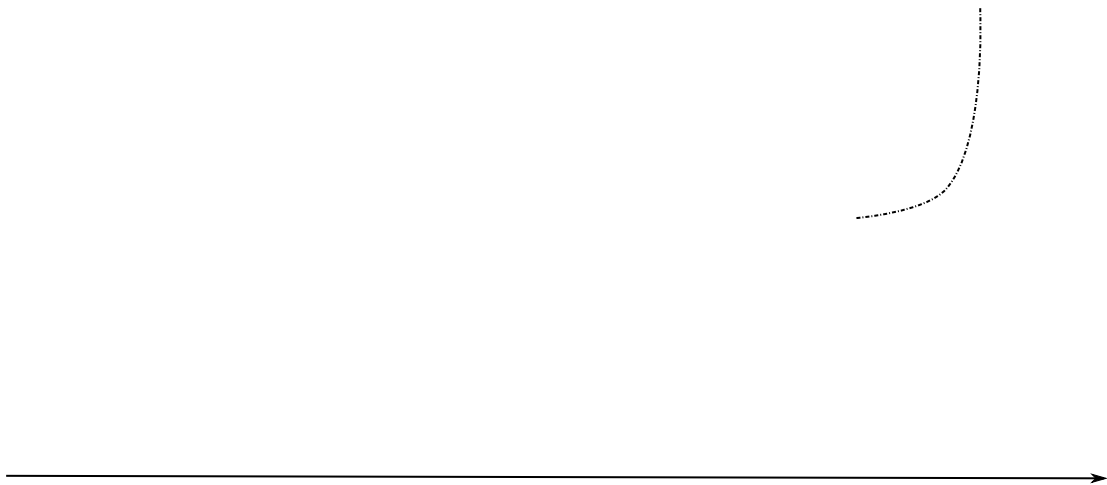

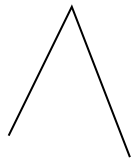

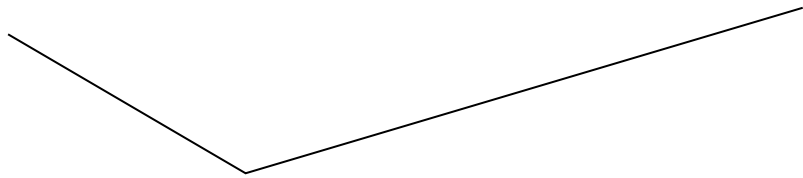

Supplement: Supplementary file 1 [file appendixfigure.pdf]
